# Supplementary material for: BP-SGCN: Behavioral Pseudo-Label Informed Sparse Graph Convolution Network for Pedestrian and Heterogeneous Trajectory Prediction
Source: arXiv:2502.14676 source file (2025-02-21)
Supplement: Supplementary file 1 [file supp.pdf]

# BP-SGCN: Behavioral Pseudo-Label Informed Sparse Graph Convolution Network for Pedestrian and Heterogeneous Trajectory Prediction – Supplementary Material

Ruochen Li<sup>✉</sup>, Stamos Katsigiannis<sup>✉</sup>, *Member, IEEE*, Tae-Kyun Kim<sup>✉</sup>, Hubert P. H. Shum<sup>✉†</sup>, *Senior Member, IEEE*

## I. MORE QUALITATIVE VISUALIZATIONS

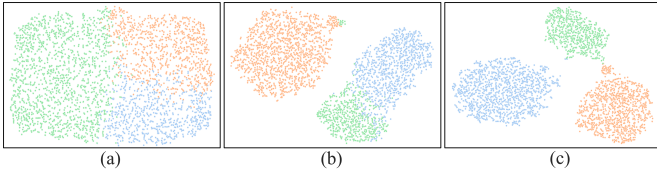

Fig. 1: The t-SNE Visualization of clustering distribution with different features on pedestrian-only SDD ( $k=3$ ), using (a) acceleration, (b) angle, and (c) acceleration + angle (ours).

In Fig. 1, we assess the quality of clustering using various geometric features. Both (a) and (b) indicate that when solely relying on acceleration or angle as input feature vectors, our unsupervised deep clustering module struggles to differentiate between the hidden representations of the three pedestrian behavioral groups. However, when combining acceleration and angle (as introduced in BP-SGCN), the distinction between these three behavioral groups becomes evident and thus leads to better trajectory prediction accuracy.

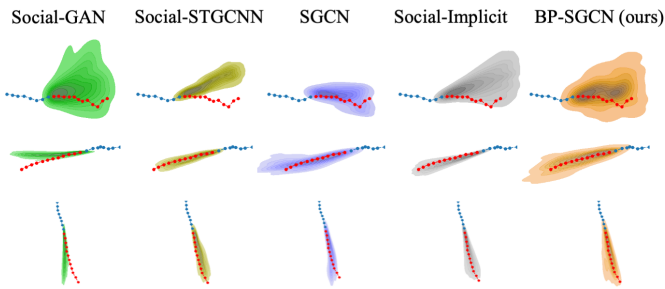

Fig. 2: Visualization of trajectory prediction on ETH/UCY of Social-GAN [1], Social-STGCNN [2], SGCN [3], Social-Implicit [4], and BP-SGCN (ours).

Fig. 2 follows the visualization scheme from [4], showcasing not only that the predicted distribution of our BP-

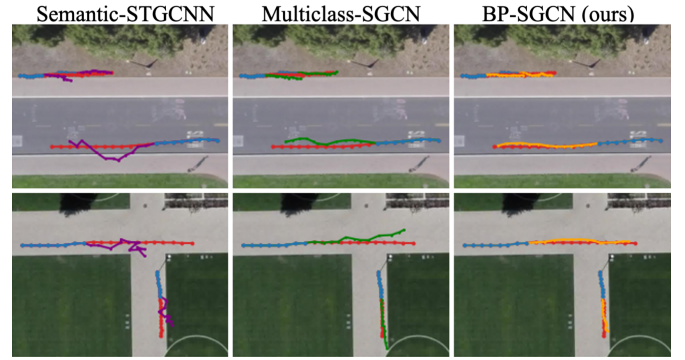

Fig. 3: The visualization of trajectory prediction on SDD of Semantic-STGCNN [5], Multiclass-SGCN [6], BP-SGCN (ours). Blue and red represent observed and ground-truth trajectories respectively, whereas other colors refer to predicted trajectories using each method.

SGCN covers whole ground-truth trajectories, but also that it provides more diverse predictions, compared to SOTA pedestrian trajectory predictions [2]–[4].

Fig. 3 visualize the trajectory prediction for heterogeneous SDD dataset. Blue and red dots represent observed and ground-truth future trajectories respectively, showcasing the superior quality of our predicted trajectories, compared to ground-truth label integrated methods [5], [6].

Fig. 4, Fig. 5 and Fig. 6 illustrate additional qualitative results on various scenes of the heterogeneous SDD dataset, heterogeneous Argoverse 1 dataset and the pedestrian-only ETH/UCY datasets, respectively. Since our model relies on sampling from a bi-variate Gaussian distribution to compute the predicted trajectory, we plot the predicted distributions instead of a single trajectory to present a comprehensive view of the prediction quality in this supplementary document.

Specifically, for the SDD dataset, we visualize the predicted trajectory distributions in real-world scenarios by overlaying them on the original background images. Fig. 4 depicts that the proposed BP-SGCN is able to predict realistic trajectory distributions that fall within valid movement areas in both simple and complex scenarios.

For Argoverse 1 dataset, Fig. 5 showcases the predictions

R. Li, S. Katsigiannis and H. P. H. Shum are with Durham University, UK. {ruochen.li, stamos.katsigiannis, hubert.shum}@durham.ac.uk

T. K. Kim is with KAIST, Korea. kimtaekyun@kaist.ac.kr

† Corresponding author: H. P. H. Shum

TABLE I: A summary of main symbols and definitions

| Symbols                    | Definition                                |
|----------------------------|-------------------------------------------|
| $p_t^i = (x_t^i, y_t^i)$   | 2D coordinates of agent $i$ at time $t$ . |
| $N$                        | Number of pedestrians                     |
| $T_{obs}$                  | Observed time steps                       |
| $T_{pred}$                 | Prediction time steps                     |
| $\mathbf{v}_t$             | Velocity vector                           |
| $\cos(\theta_t)$           | Cosine of the angle                       |
| $ \mathbf{a}_t $           | Magnitude of acceleration                 |
| $g_t$                      | Agent geometric feature                   |
| $\varphi_{enc}$            | Encoder network of VRNN                   |
| $h$                        | Recurrent hidden state                    |
| $q_\phi$                   | Posterior distribution                    |
| $\varphi_{dec}$            | Decoder network of VRNN                   |
| $p_\delta$                 | Reconstruction distribution               |
| $\varphi_{prior}$          | Prior distribution                        |
| $\mathcal{L}_{VRNN}$       | Loss of VRNN                              |
| $\mathcal{L}_{Soft-DTW}$   | Loss of soft-DTW                          |
| $\mathcal{L}_{ELBO}$       | Loss of ELBO                              |
| $q$                        | Q Distribution for soft assignment        |
| $p$                        | Auxiliary distribution P                  |
| $\mathcal{L}_{cluster}$    | Loss of deep clustering                   |
| $f$                        | Soft cluster frequency                    |
| $l$                        | Agent class label                         |
| $\mathcal{G}_s$            | Spatial graph                             |
| $\mathcal{V}_s$            | Node of $\mathcal{G}_s$                   |
| $\mathcal{A}_s$            | Adjacency matrix of $\mathcal{G}_s$       |
| $\mathcal{G}_t$            | Temporal graph                            |
| $\mathcal{V}_t$            | Node of $\mathcal{G}_t$                   |
| $\mathcal{A}_t$            | Adjacency matrix of $\mathcal{G}_t$       |
| $\mathcal{L}_{prediction}$ | Loss of bi-variate Gaussian distribution  |
| $\mathcal{L}_{final}$      | Combined loss                             |

generated by our model adhering to the map. In straightforward scenarios, BP-SGCN effectively forecasts trajectories with varied speed profiles. When faced with intersections, the model offers multimodal predictions, capturing the potential intentions of the agents.

For the ETH/UCY datasets, we visualize the trajectory distribution across scenarios, ranging from simple to complex scenarios (from top row to bottom row). Fig. 6 demonstrates that BP-SGCN capably produces realistic pedestrian trajectory predictions across varied social contexts.

Notably, there are some sub-optimal results shown in the visualizations if the number of agents is large, mainly due to the randomness of agent movements. However, the proposed BP-SGCN can still provide plausible trajectory distribution predictions in these cases, as the predicted trajectory distributions can almost cover the ground-truth trajectories. Overall, the provided trajectory prediction visualizations demonstrate the effectiveness of the proposed BP-SGCN for heterogeneous and pedestrian-only trajectory prediction in diverse traffic scenarios.

## II. SUMMARY OF NOTATIONS

TABLE I includes the definitions of main symbols used in the proposed method.

## REFERENCES

- [1] A. Gupta, J. Johnson, L. Fei-Fei, S. Savarese, and A. Alahi, “Social gan: Socially acceptable trajectories with generative adversarial networks,” in *Proc. IEEE/CVF Conf. Comput. Vis. Pattern Recognit.*, 2018, pp. 2255–2264. [1](#)
- [2] A. Mohamed, K. Qian, M. Elhoseiny, and C. Claudel, “Social-stgcnn: A social spatio-temporal graph convolutional neural network for human trajectory prediction,” in *Proc. IEEE/CVF Conf. Comput. Vis. Pattern Recognit.*, 2020, pp. 14 424–14 432. [1](#)
- [3] L. Shi, L. Wang, C. Long, S. Zhou, M. Zhou, Z. Niu, and G. Hua, “Sgcn: Sparse graph convolution network for pedestrian trajectory prediction,” in *Proc. IEEE/CVF Conf. Comput. Vis. Pattern Recognit.*, 2021, pp. 8994–9003. [1](#)
- [4] A. Mohamed, D. Zhu, W. Vu, M. Elhoseiny, and C. Claudel, “Social-implicit: Rethinking trajectory prediction evaluation and the effectiveness of implicit maximum likelihood estimation,” in *Proc. Eur. Conf. Comput. Vis.*, 2022, pp. 463–479. [1](#)
- [5] B. A. Rainbow, Q. Men, and H. P. Shum, “Semantics-stgcnn: A semantics-guided spatial-temporal graph convolutional network for multi-class trajectory prediction,” in *IEEE Int. Conf. Syst. Man Cybern.* IEEE, 2021, pp. 2959–2966. [1](#)
- [6] R. Li, S. Katsigiannis, and H. P. Shum, “Multiclass-sgcn: Sparse graph-based trajectory prediction with agent class embedding,” in *IEEE Int. Conf. Image Process.* IEEE, 2022, pp. 2346–2350. [1](#)

[1] A. Gupta, J. Johnson, L. Fei-Fei, S. Savarese, and A. Alahi, “Social gan: Socially acceptable trajectories with generative adversarial networks,” in

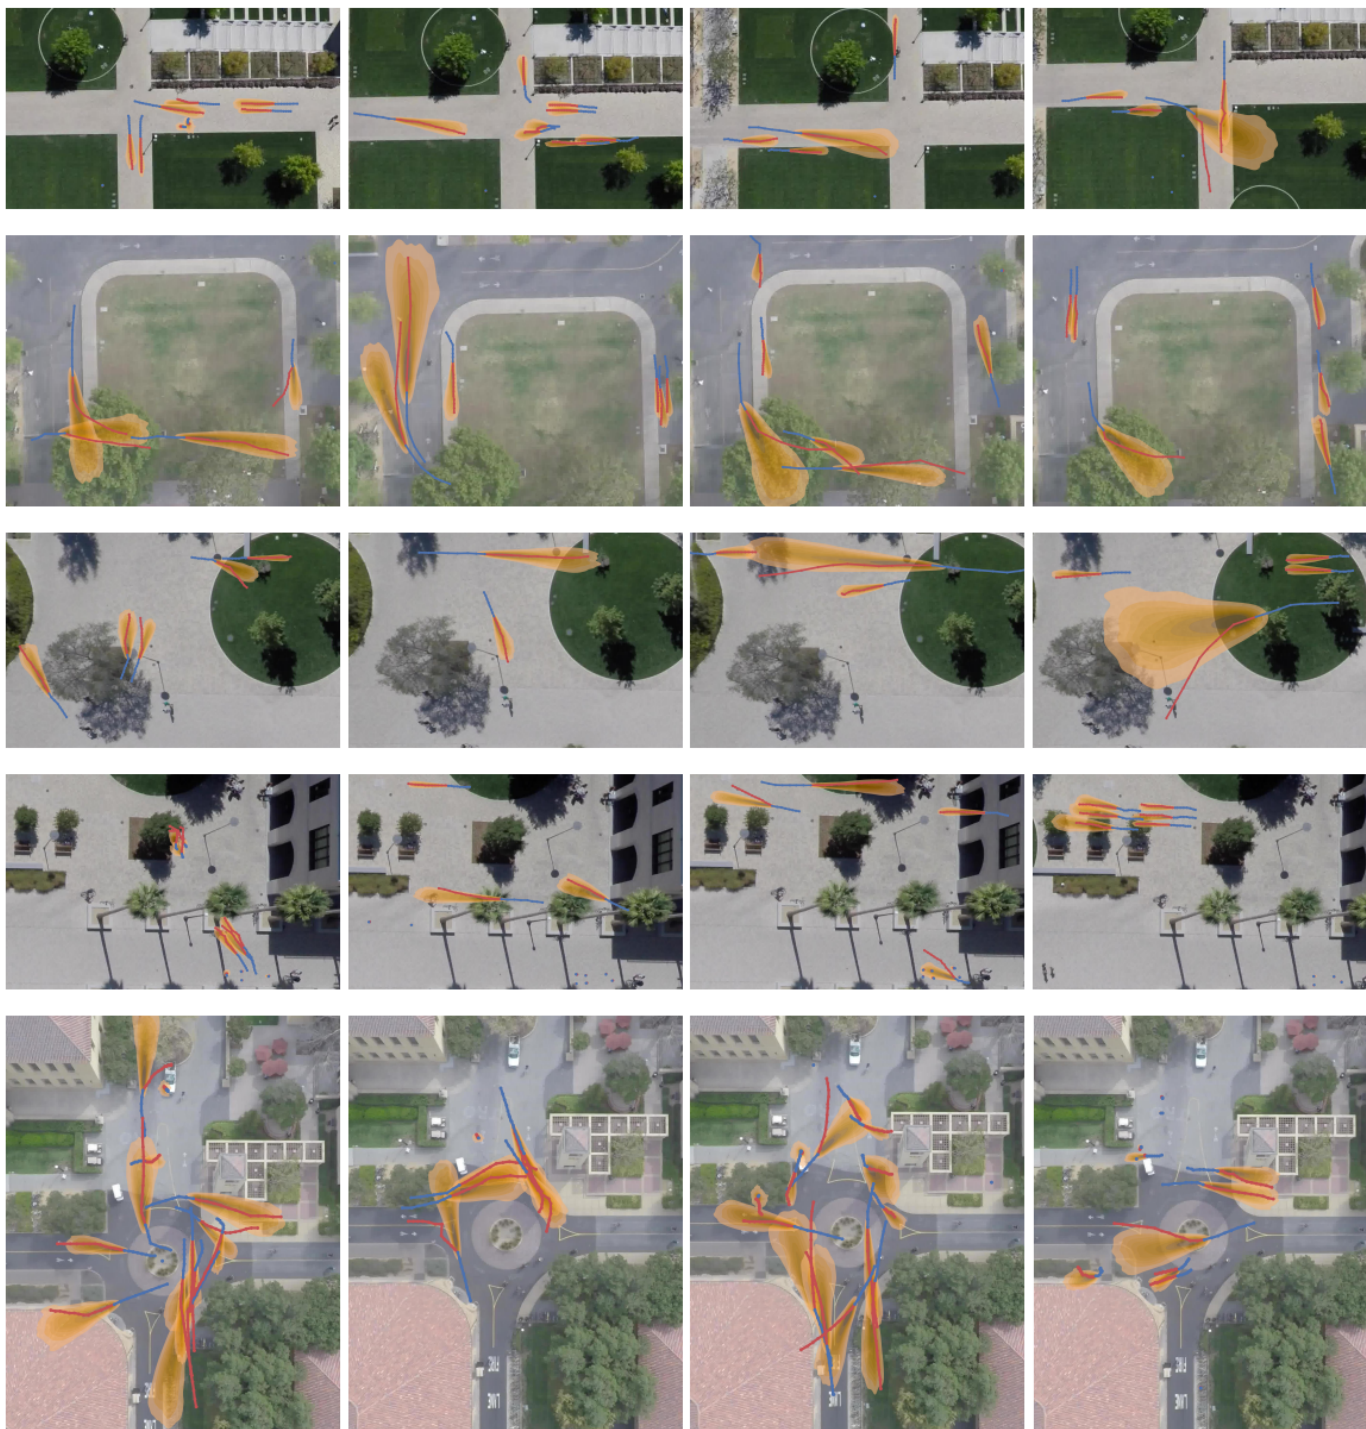

Fig. 4: Predicted trajectory distributions using the proposed BP-SGCN on the SDD dataset. Past trajectories are shown in blue, ground-truth trajectories in red, and predicted trajectory distributions in orange.

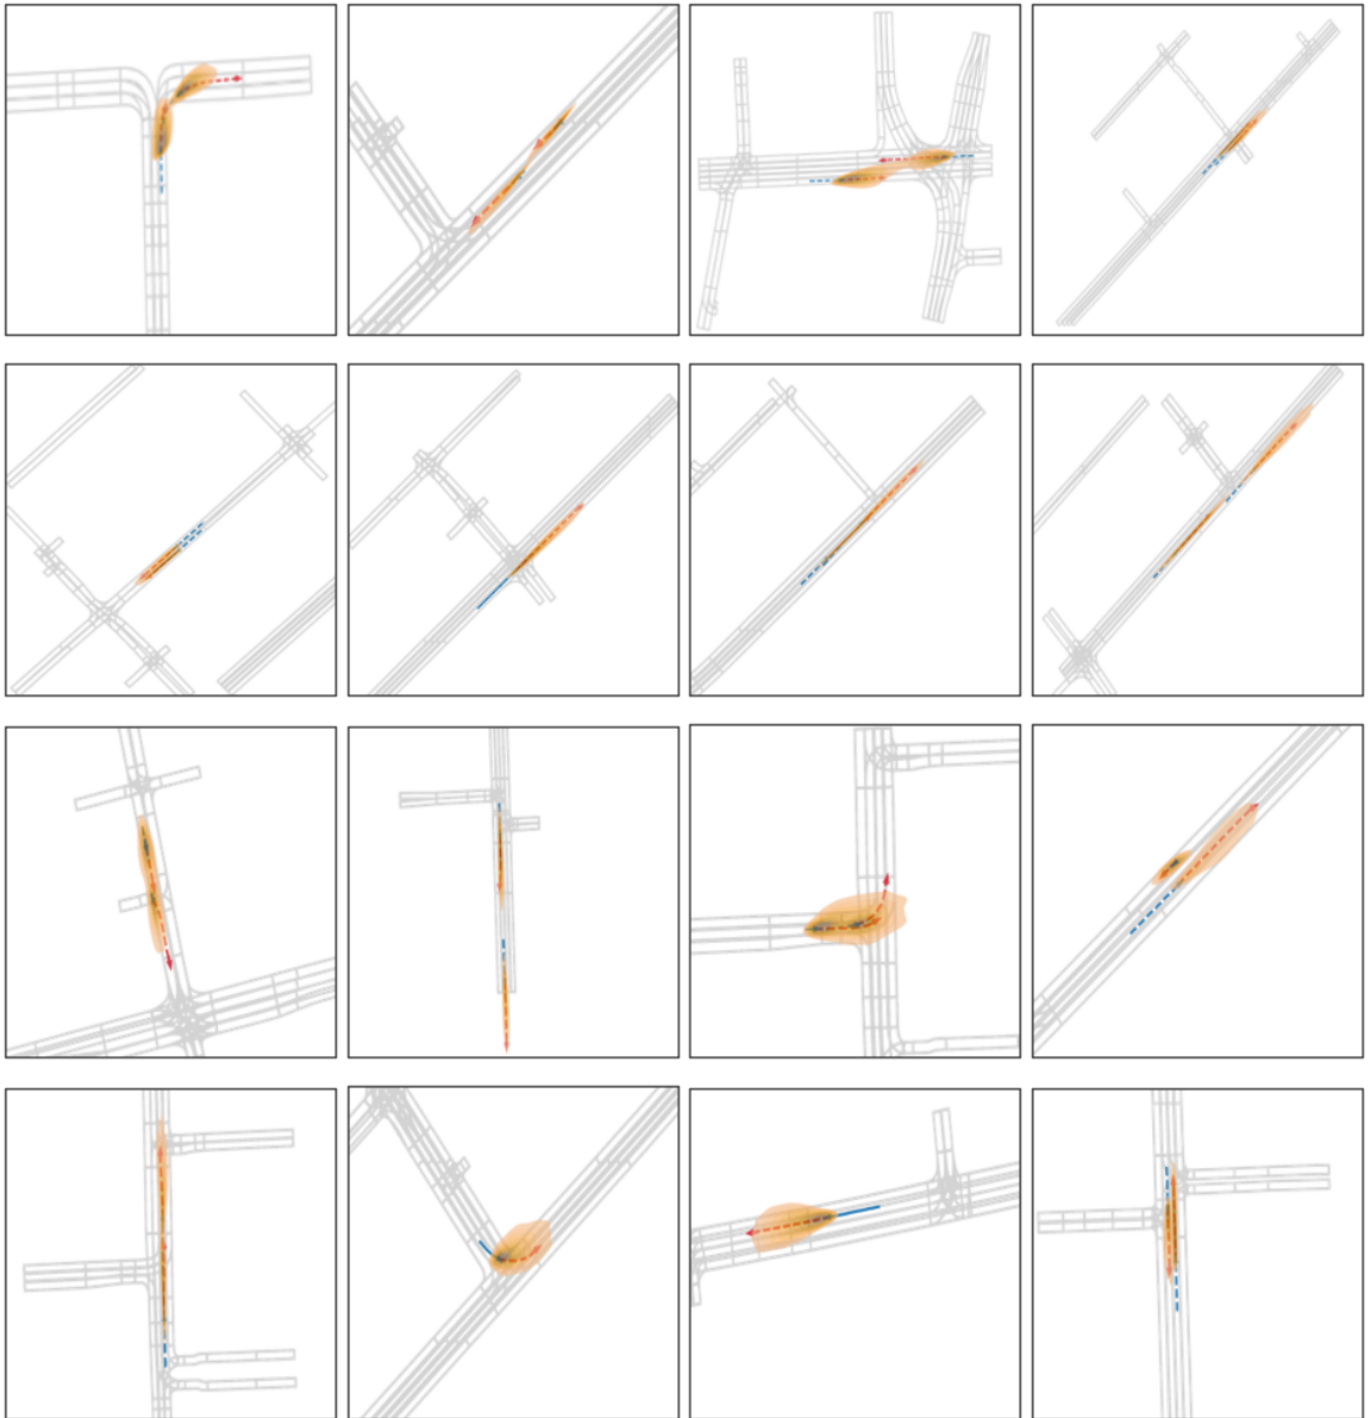

Fig. 5: Predicted trajectory distributions using the proposed BP-SGCN on the Argoverse 1 dataset. Past trajectories are shown in blue, ground-truth trajectories in red, and predicted trajectory distributions in orange.

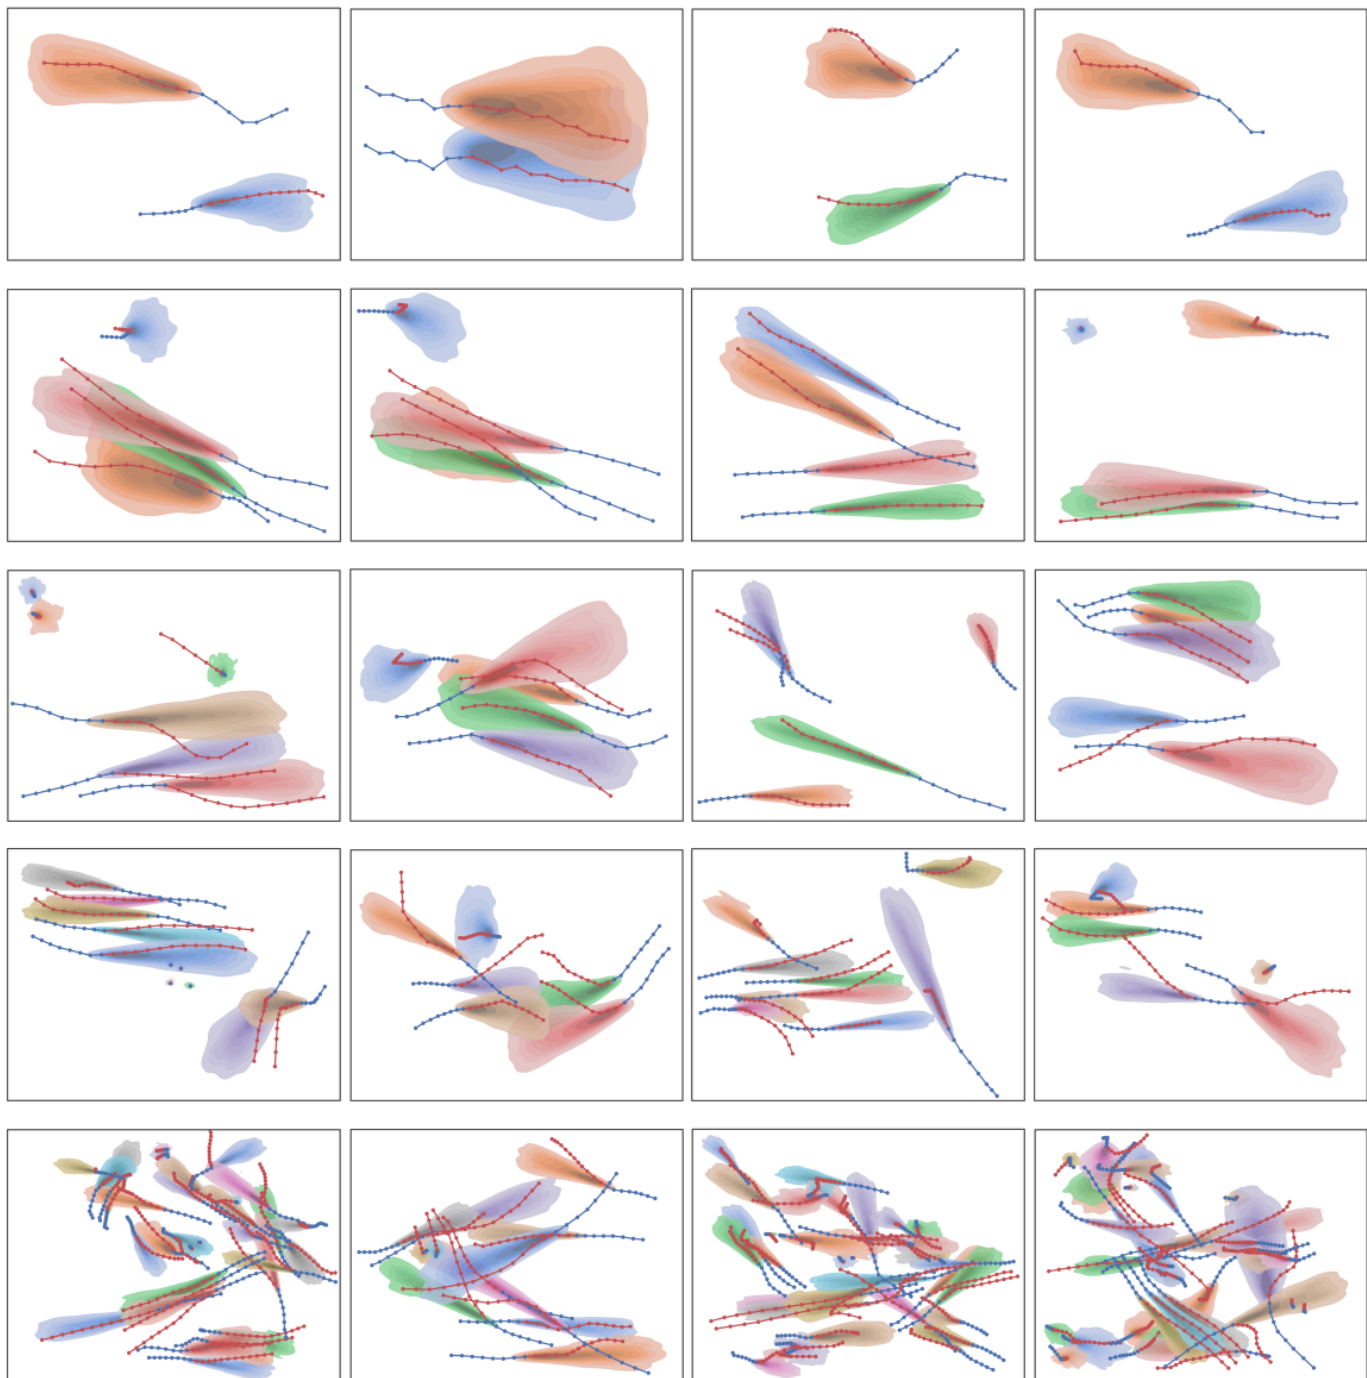

Fig. 6: Predicted trajectory distributions using the proposed BP-SGCN on the ETH/UCY datasets. The complexity level of social interactions among pedestrians increases from the top row to the bottom row. Past trajectories are shown in blue and ground-truth trajectories are shown in red. Due to the relatively high pedestrian density, we use different colors to represent the predicted trajectory distributions of different pedestrians
